# Supplementary material for: Repo2Vec: A Comprehensive Embedding Approach for Determining Repository Similarity
Source: arXiv:2107.05112 source file (2021-07-11)
Supplement: Supplementary file 1 [file 070appendix.tex]

%%%%%%%%%%%%%%%%%%%%%%%%%%%%%%%%%%%%%%%
% AUTHOR: Christos Faloutsos
% INSTITUTION: CMU
% DATE: April 2019
% GOAL: to streamline the paper presentations
%%%%%%%%%%%%%%%%%%%%%%%%%%%%%%%%%%%%%%%

\section{Stealth appendix}
\reminder{[here we put self notes etc, that we will NOT include
in the final paper]}
